# Supplementary material for: A full gap above the Fermi level: the charge density wave of monolayer VS2
Source: arXiv:2101.01140 source file (2021-09-08)
Supplement: Supplementary file 1 [file supplement.tex]

\documentclass[10pt]{nature}

\pdfoutput=1

\usepackage[english]{babel}
\usepackage{graphicx}
\graphicspath{{Sfig/}}
\usepackage{siunitx}
\usepackage{mathtools}
\usepackage{microtype}
\usepackage[dvipsnames, pdftex]{xcolor}
\usepackage{xr}
\externaldocument[art:]{article}
\usepackage[labelfont=bf, textfont=md]{caption}
\usepackage[pdftex, colorlinks, allcolors=blue]{hyperref}

\let\vec\boldsymbol

\newcommand{\va}{VS\textsubscript2}
\newcommand{\ve}{VSe\textsubscript2}

\newcommand{\ta}{TaS\textsubscript2}

\newcommand{\vte}{VTe\textsubscript2}

\newcommand{\1}{$1 \times 1$}

\newcommand{\3}{$3 \times 3$}
\newcommand{\4}{$4 \times 4$}

\newcommand{\7}{$7 \times \sqrt 3 \mathrm R30^\circ$}
\newcommand{\9}{$9 \times \sqrt 3 \mathrm R30^\circ$}
\newcommand{\dIdV}{$\mathrm d I / \mathrm d V$}

\setlength\parskip{6pt}

\begin{document}

\title{Supplementary Information of ``A full gap above the Fermi level: the charge density wave of monolayer \va''}
\maketitle
\author{Camiel van Efferen$^1*$,}
\author{Jan Berges$^2$,}
\author{Joshua Hall$^1$,}
\author{Erik van Loon$^2$,}
\author{Stefan Kraus$^{1}$,}
\author{Arne Schobert$^2$,}
\author{Tobias Wekking$^{1}$,}
\author{Felix Huttmann$^{1}$,}
\author{Eline Plaar$^1$,}
\author{Nico Rothenbach$^3$,}
\author{Katharina Ollefs$^3$,}
\author{Lucas Machado Arruda$^4$,}
\author{Nick Brookes$^5$,}
\author{Gunnar Sch\"{o}nhoff$^2$,}
\author{Kurt Kummer$^5$,}
\author{Heiko Wende$^3$,}
\author{Tim Wehling$^2$,}
\author{Thomas Michely$^1$}

\begin{affiliations}
\item II. Physikalisches Institut, Universit\"at zu K\"oln, Z\"ulpicher Stra\ss e 77, 50937 K\"oln, Germany
\item Institut f\"ur Theoretische Physik, Bremen Center for Computational Materials Science, and MAPEX Center for Materials and Processes, Otto-Hahn-Allee 1, Universit\"at Bremen, 28359 Bremen, Germany
\item Fakult\"at f\"ur Physik und Center f\"ur Nanointegration Duisburg-Essen (CENIDE), Universit\"at Duisburg-Essen, Carl-Benz-Stra\ss e, 47057 Duisburg, Germany
\item Institut f\"ur Experimentalphysik, Freie Universit\"at Berlin, Arnimallee 14, 14195 Berlin, Germany
\item European Synchrotron Research Facility (ESRF), Avenue des Martyrs 71, CS 40220, 38043 Grenoble Cedex 9, France
\end{affiliations}

\pagebreak

\section*{Figure~\ref*{fig:UnitCells}: Unit cells}

\begin{figure*}[h!]
\centering
\includegraphics[width=0.98\columnwidth]{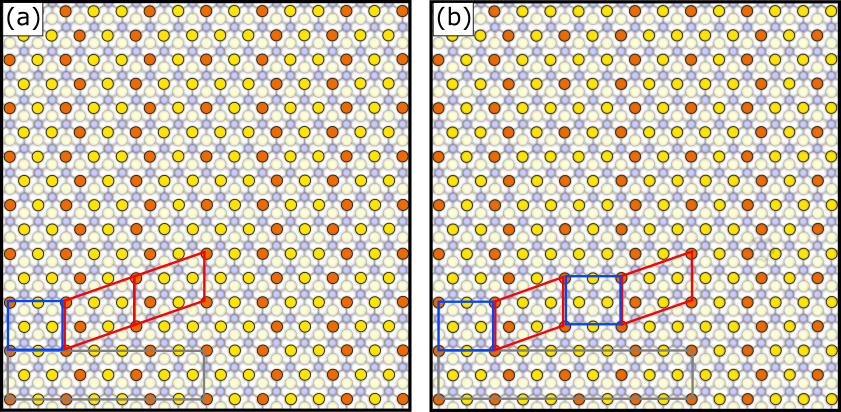}
\caption{Correspondence between unit cells in monolayer \ve{} literature and the unit cells used in this paper. In \textbf a and \textbf b, models of the 1T-\va{} atomic lattice are depicted with V atoms in blue and bottom-S atoms in faint yellow. \7 (\textbf a) and \9 (\textbf b) superstructures are visible in the top-S atoms, which are drawn in two colors to mimic the experimental apparent height in yellow (bright) and orange (dark). The dark gray rectangles indicate the \7 (\textbf a) and \9 (\textbf b) unit cells. The blue rectangle is a $2 \times \sqrt{3}$R30$^{\circ}$ unit, the red rhombus a $\sqrt{7}$R19.1$^{\circ} \times \sqrt{3}$R30$^{\circ}$.}
 \label{fig:UnitCells}
\end{figure*}

\noindent
In the isotypic material \ve, a superstructure of same symmetry as in \va{}, has been identified and attributed to a charge density wave (CDW)\cite{Duvjir2018, Chen2018, Coelho2019, Wong2019}. In these studies, the superstructure was described by a combination of $2 \times \sqrt{3}$R30$^{\circ}$ and $\sqrt{7}$R19.1$^{\circ} \times \sqrt{3}$R30$^{\circ}$ units, which we mark in our model in Fig.~\ref{fig:UnitCells}a,\,b in blue and red, respectively. By the combination of a single $2 \times \sqrt{3}$R30$^{\circ}$ and two $\sqrt{7}$R19.1$^{\circ} \times \sqrt{3}$R30$^{\circ}$ units, the \7 CDW lattice can be described; two $2 \times \sqrt{3}$R30$^{\circ}$ units and two $\sqrt{7}$R19.1$^{\circ} \times \sqrt{3}$R30$^{\circ}$ units make up the \9 lattice.

\pagebreak

\section*{Figure~\ref*{fig:VS2CDWSTMTip}: Tip-induced switching between distorted and undistorted phase}

\begin{figure*}[h!]
\centering
\includegraphics[width=\columnwidth]{fig02.png}
\caption{Influence of STM tip on monolayer \va: the two consecutive STM scans in panel \textbf a and \textbf b document the STM-tip-induced switch from the undistorted to the superstructure CDW phase. Scan \textbf c is taken 15 minutes later and shows no more signs of the superstructure. Images taken at \SI{300}{\kelvin}. Measurement parameters: \textbf{a--c}~\SI[parse-numbers=false]{7 \times 7}{\nano\meter\squared}, $I_{\text{t}} = \SI{0.5}{\nano\ampere}$, $V_{\text{t}} = \SI{-90}{\meV}$.}
 \label{fig:VS2CDWSTMTip}
\end{figure*}

\noindent
The presence of the superstructure at room temperature can also be influenced by the scanning tunneling microscope (STM) tip. Figure~\ref{fig:VS2CDWSTMTip}a,\,b shows two consecutive STM scans, taken at the same position, tunnelling current, and bias. In Fig.~\ref{fig:VS2CDWSTMTip}a, the STM reveals only hexagonal atomic ordering inside the small \va{} structure. In the successive STM scan in Fig.~\ref{fig:VS2CDWSTMTip}b, the wave superstructure is observed in the same region, with the phase transition apparently triggered by the interaction with the STM tip. A subsequent STM scan taken about 15 minutes later, displayed in Fig.~\ref{fig:VS2CDWSTMTip}c, again shows the absence of the superstructure.

\pagebreak

\section*{Figure~\ref*{fig:vse2}: 1T-\ve{} vs 1T-\va{} and \9 vs \7}

\begin{figure*}[h!]
\centering
\includegraphics[width=\linewidth]{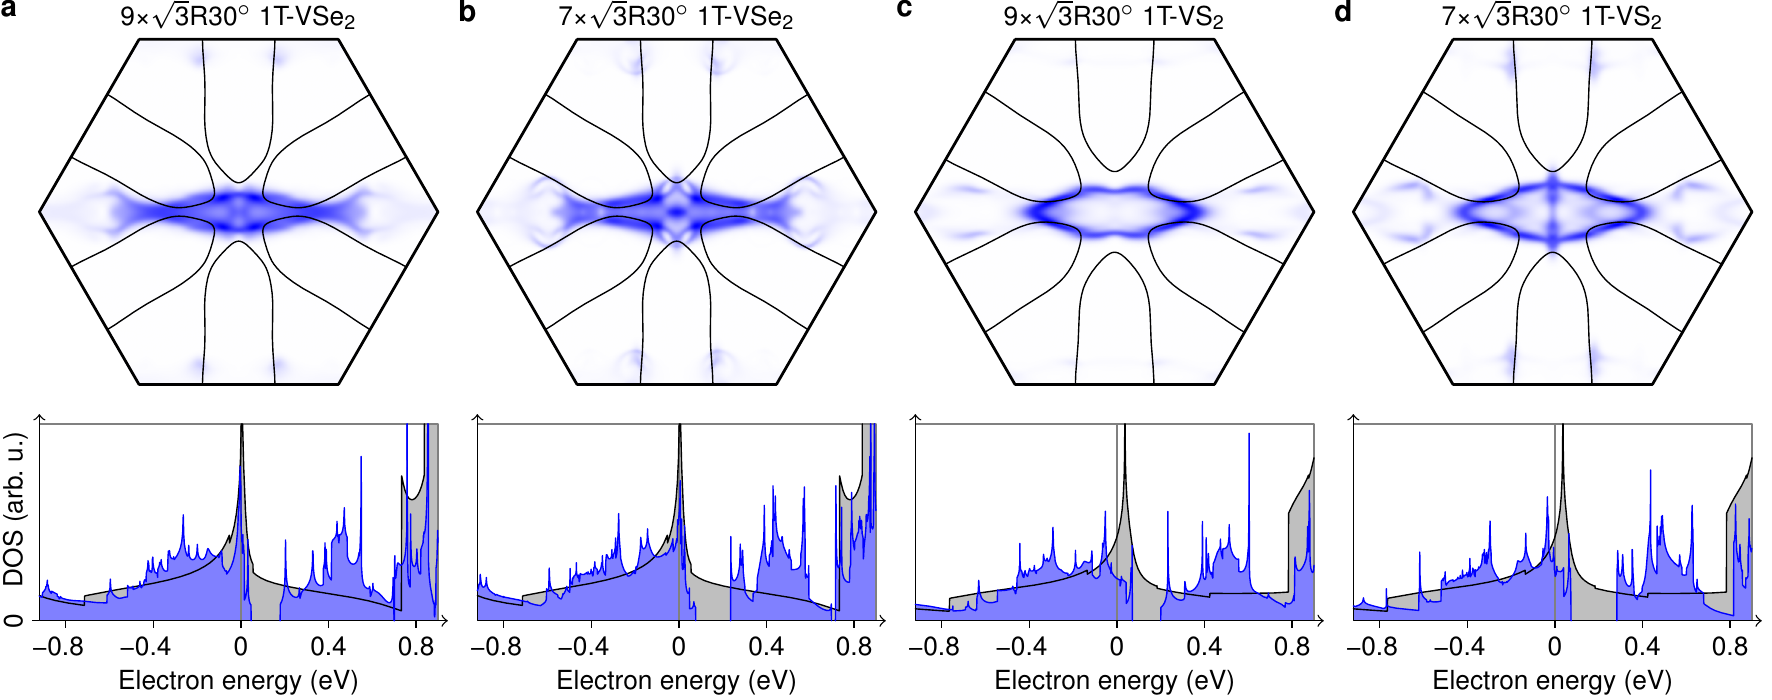}
\caption{Fermi surface and DOS of monolayer \textbf{a,\,b}~1T-\ve{} and \textbf{c,\,d}~1T-\va{} in the undistorted phase as well as for the \textbf{a,\,c}~\9 and \textbf{b,\,d}~\7 CDW as obtained from DFT\@. The CDW data has been unfolded to the Brillouin zone of the undistorted structure. Here, the color saturation corresponds to the overlap of CDW and undistorted wave functions for the same $\vec k$ point.}
 \label{fig:vse2}
\end{figure*}

\noindent
In Fig.~\ref{fig:vse2}a,\,b, we show the Fermi surface and density of states (DOS) of monolayer 1T-\ve{} in the undistorted as well as \9 and \7 CDW phases from density functional theory (DFT). In \ve{} a similar CDW as the one found in \va{} has been reported repeatedly\cite{Bonilla2018, Chen2018, Wong2019, Duvjir2018, Chua2020}. As points of reference, corresponding results for monolayer 1T-\va{} are displayed in Fig.~\ref{fig:vse2}c,\,d. The results for the \9 and \7 cells agree qualitatively. Furthermore, our calculations suggest that 1T-\ve{} and 1T-\va{} are very similar in their electronic structure. In the distorted phase, 1T-\ve{} will also have a full gap in the unoccupied states; at the Fermi energy, only a partial gap is expected. Though this has been observed in experiment\cite{Chen2018, Coelho2019}, most studies on monolayer \ve{} agree on a full gap located at the Fermi level\cite{Feng2018, Duvjir2018, Wong2019, Chua2020}. To our understanding, such a gap would require a filling of the downwards-dispersing bands near $\Gamma$, which are not gapped in the CDW configuration. According to our DFT calculations for both 1T-\va{} and 1T-\ve{} on a \9 (\7) supercell, $1/9 \approx 0.11$ ($1/7 \approx 0.14$) additional electrons would shift the gap to the Fermi energy (compare Fig.~\ref{fig:avoided_crossing}a,\,b). This charge could be provided by, e.g., the substrate or defects.

\pagebreak

\section*{Figure~\ref*{fig:FSN}: Nesting conditions and electron--phonon coupling}

\begin{figure*}[h!]
\centering
\includegraphics[width=\linewidth]{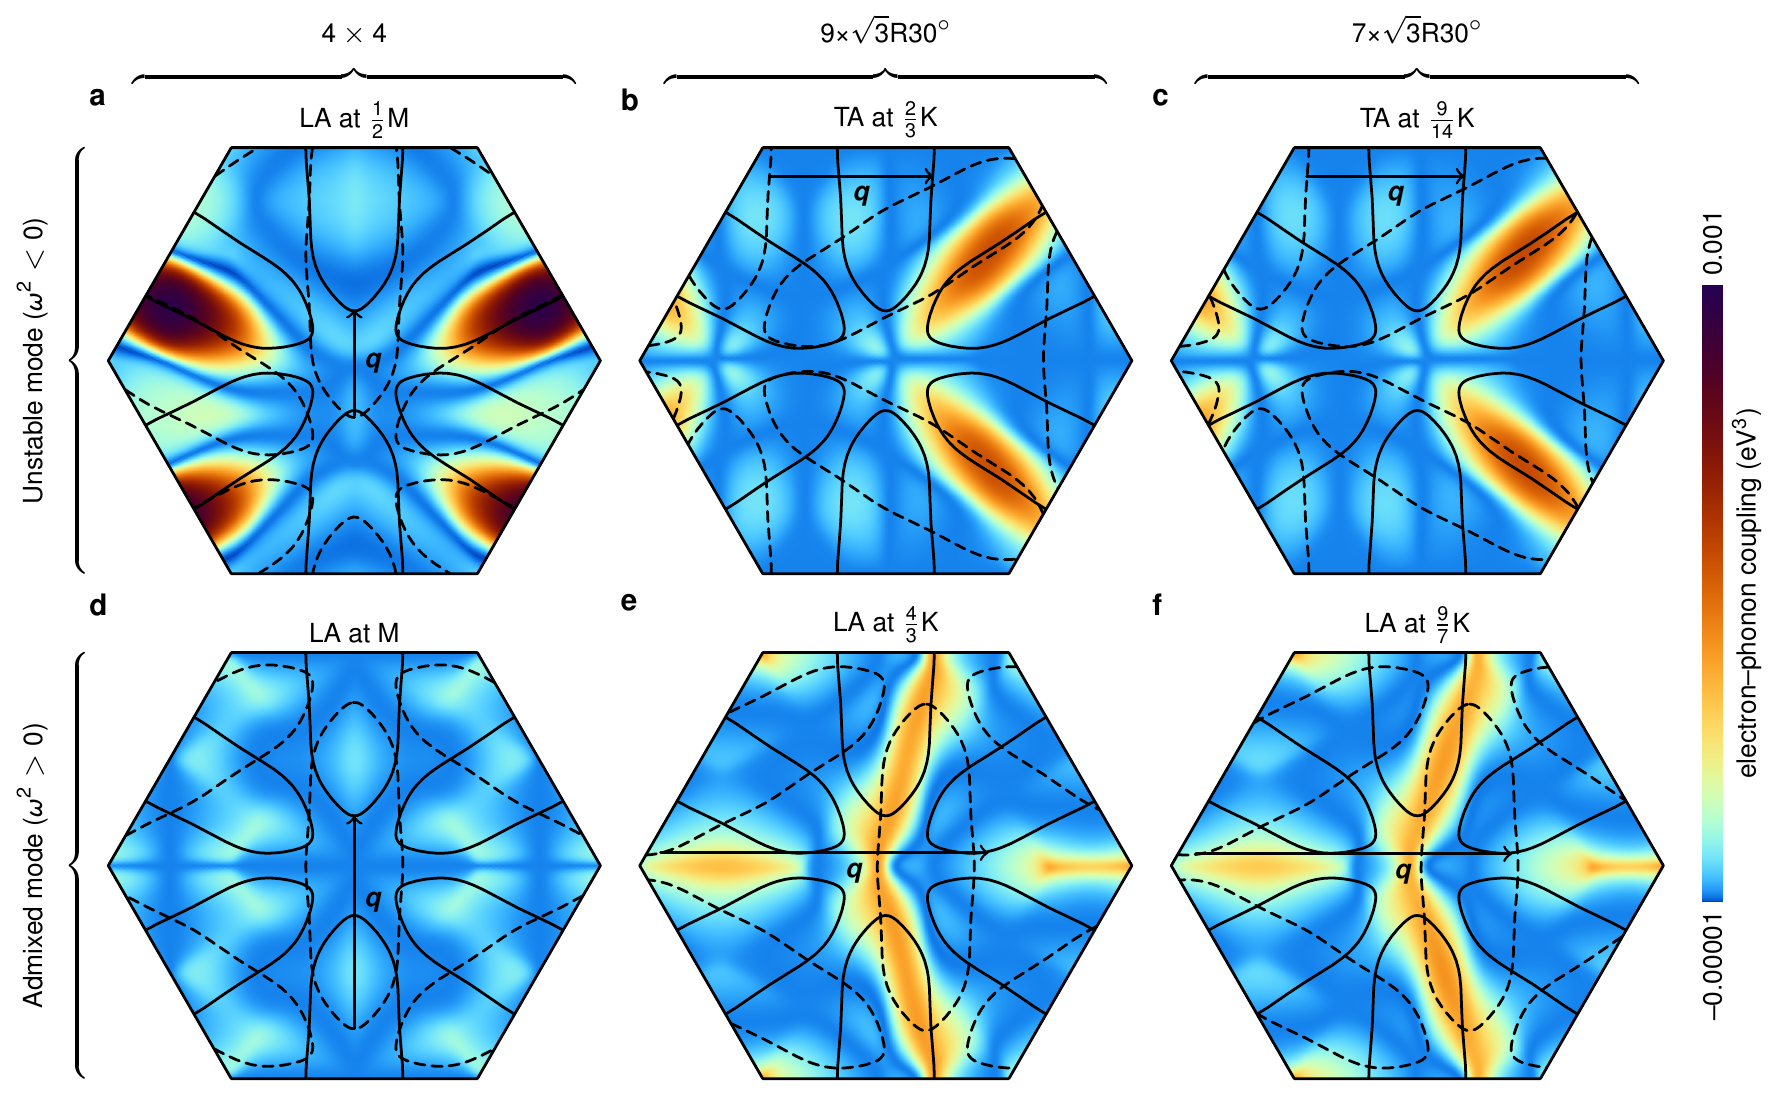}
\caption{Nesting conditions for different phonon wavevectors $\vec q$. We show the relevant electron--phonon coupling $2 \omega_{\vec q} g_{\vec k + \vec q, \vec k} \widetilde g_{\vec k, \vec k + \vec q}$ as a function of the electron wavevector $\vec k$ (color scale) together with the original Fermi surface (solid lines) and the Fermi surface shifted by $-\vec q$ (dashed lines). Nesting parts of the Fermi surface can only have a strong effect on the phonons if they occur in $\vec k$-space regions with significant electron--phonon coupling (dark/brown spots). While the $\widetilde g$ from DFPT is fully screened, the partially screened $g$ from constrained DFPT (cDFPT)\cite{Nomura2015} excludes low-energy electronic screening (precisely, from within the isolated band at the Fermi level). Together with the bare electronic susceptibility $\chi_0$, they determine the phonon self-energy $\varPi = g^* \chi_0 \widetilde g$ responsible for the instabilities in the phonon dispersion. This analysis is equivalent to the fluctuation diagnostics in Ref.~\citenum{Berges2020}. The electron--phonon coupling has been obtained via the EPW code\cite{Giustino2007, Ponce2016}.}
 \label{fig:FSN}
\end{figure*}

\noindent
In Fig.~2a of the manuscript, we can observe two main instabilities in the acoustic phonon dispersion of monolayer 1T-\va from density functional perturbation theory (DFPT): one in the longitudinal branch at $\vec q \approx 1/2\,\overline{\Gamma \mathrm M}$ and one in the transverse branch at $\vec q \approx 2/3\,\overline{\Gamma \mathrm K}$. A mode with momentum $\vec q$ will be favoured if there is a large electron--phonon coupling matrix element connecting momenta $\vec k$ and $\vec k + \vec q$ close to the Fermi surface. These nesting conditions are investigated in Fig.~\ref{fig:FSN}. In the longitudinal case, shown in Fig.~\ref{fig:FSN}a, we have almost perfect Fermi-surface nesting together with a strong electron--phonon coupling (cf.~Fig.~5c,\,d of Ref.~\citenum{Chua2021} for the case of 1T-\ve). This $\vec q$ point is compatible with the formation of a $4 \times 4$ CDW, as found, e.g., in bulk \ve\cite{Williams1976}. Interestingly, despite these favorable conditions, this is not the preferred ground state of monolayer \va. Instead, a CDW with a wavevector near $\vec q = 2/3\,\overline{\Gamma \mathrm K}$ and $\vec q = 9/14\,\overline{\Gamma \mathrm K}$ develops, which features only approximate nesting and a slightly reduced coupling strength, as seen in Fig.~\ref{fig:FSN}b,\,c. As discussed in the main text, the formation of the CDW can only be understood considering non-linear mode--mode coupling. Phonon modes that appear stable in the harmonic approximation contribute significantly to the final atomic displacements, especially the longitudinal--acoustic modes for twice the momenta of the unstable modes, i.e., $\vec q = \mathrm M$, $\vec q = 9/7\,\overline{\Gamma \mathrm K}$, and $\vec q = 4/3\,\overline{\Gamma \mathrm K}$, see Fig.~\ref{fig:FSN}d--f. For both the harmonic (Fig.~\ref{fig:FSN}b,\,c) and the higher-order contributions (Fig.~\ref{fig:FSN}e,\,f) to the experimentally observed CDW, we find a similar situation of partially overlapping Fermi pockets in $\vec k$-space regions of considerable coupling, except that different pairs of pockets are involved.

\pagebreak

\section*{Figure~\ref*{fig:TaS2}: Born--Oppenheimer energy surface in \ta}

\begin{figure*}[h!]
\centering
\includegraphics[width=\linewidth]{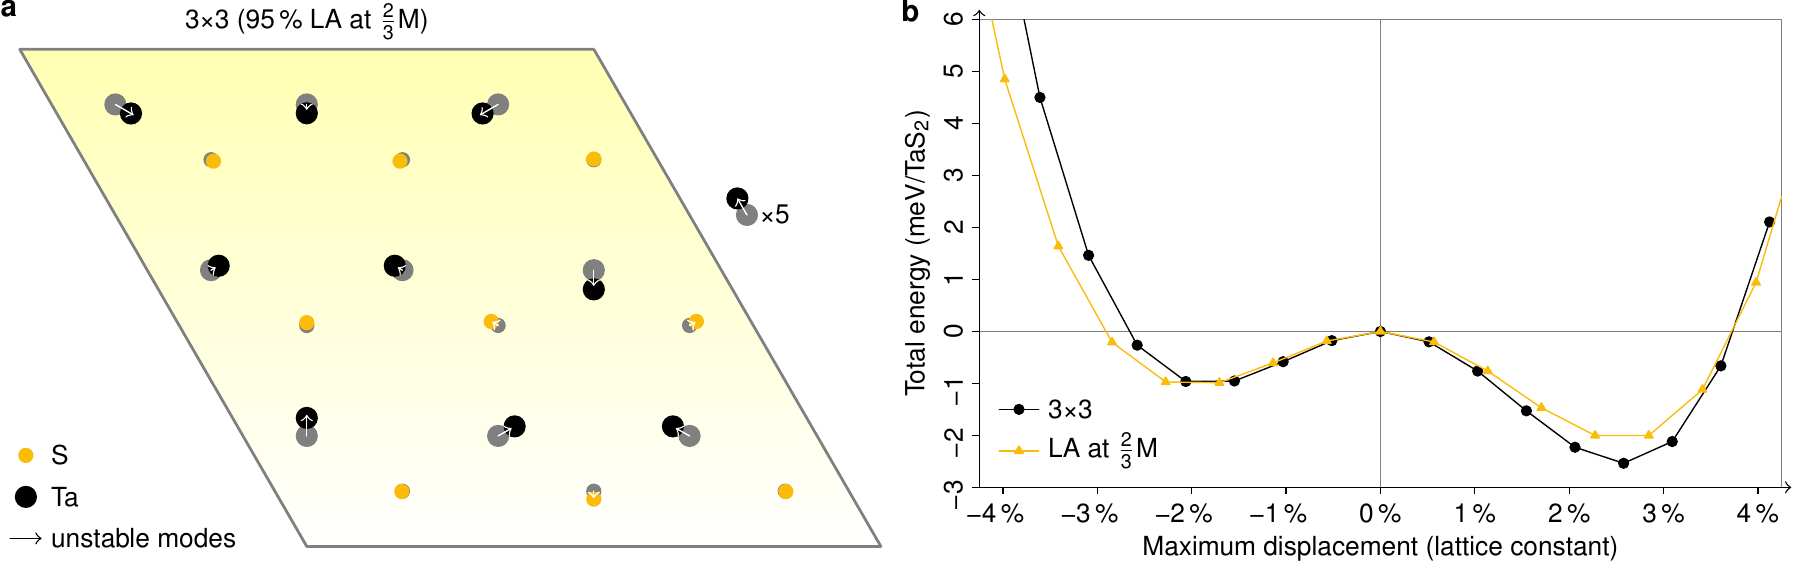}
\caption{\textbf a~CDW distortion in monolayer 2H-\ta{} and \textbf b~corresponding Born--Oppenheimer energy surface. Full circles indicate atomic positions and energies for displacements in the direction of the relaxed structure, arrows and triangle marks those for the projection onto the unstable longitudinal--acoustic phonon modes at the six wavevectors $\vec q = 2/3\,\overline{\Gamma \mathrm M}$. The relaxed atomic displacements have been amplified by a factor of five for better visibility.}
 \label{fig:TaS2}
\end{figure*}

\noindent
While the experimentally observed CDW in \va{} can only be explained by the nonlinear coupling between soft and stable phonon modes, the \3 CDW in the trigonal--prismatic TMDCs is an example of a lattice instability that is determined essentially by a single unstable phonon mode. Analogous to Fig.~2b--e, Fig.~\ref{fig:TaS2} shows the \3 CDW structure and the corresponding Born--Oppenheimer energy surface of monolayer 2H-\ta{} from DFT: Here, the distortion along the leading unstable phonon normal-mode coordinate largely captures the energy gain associated with the full CDW relaxation. We used the same computational parameters as in Ref.~\citenum{Berges2020}.

\pagebreak

\section*{Figure~\ref*{fig:VTe2}: Phonon dispersion, nesting conditions, and electron--phonon coupling in 1T-\vte}

\begin{figure*}[h!]
\centering
\includegraphics[width=\linewidth]{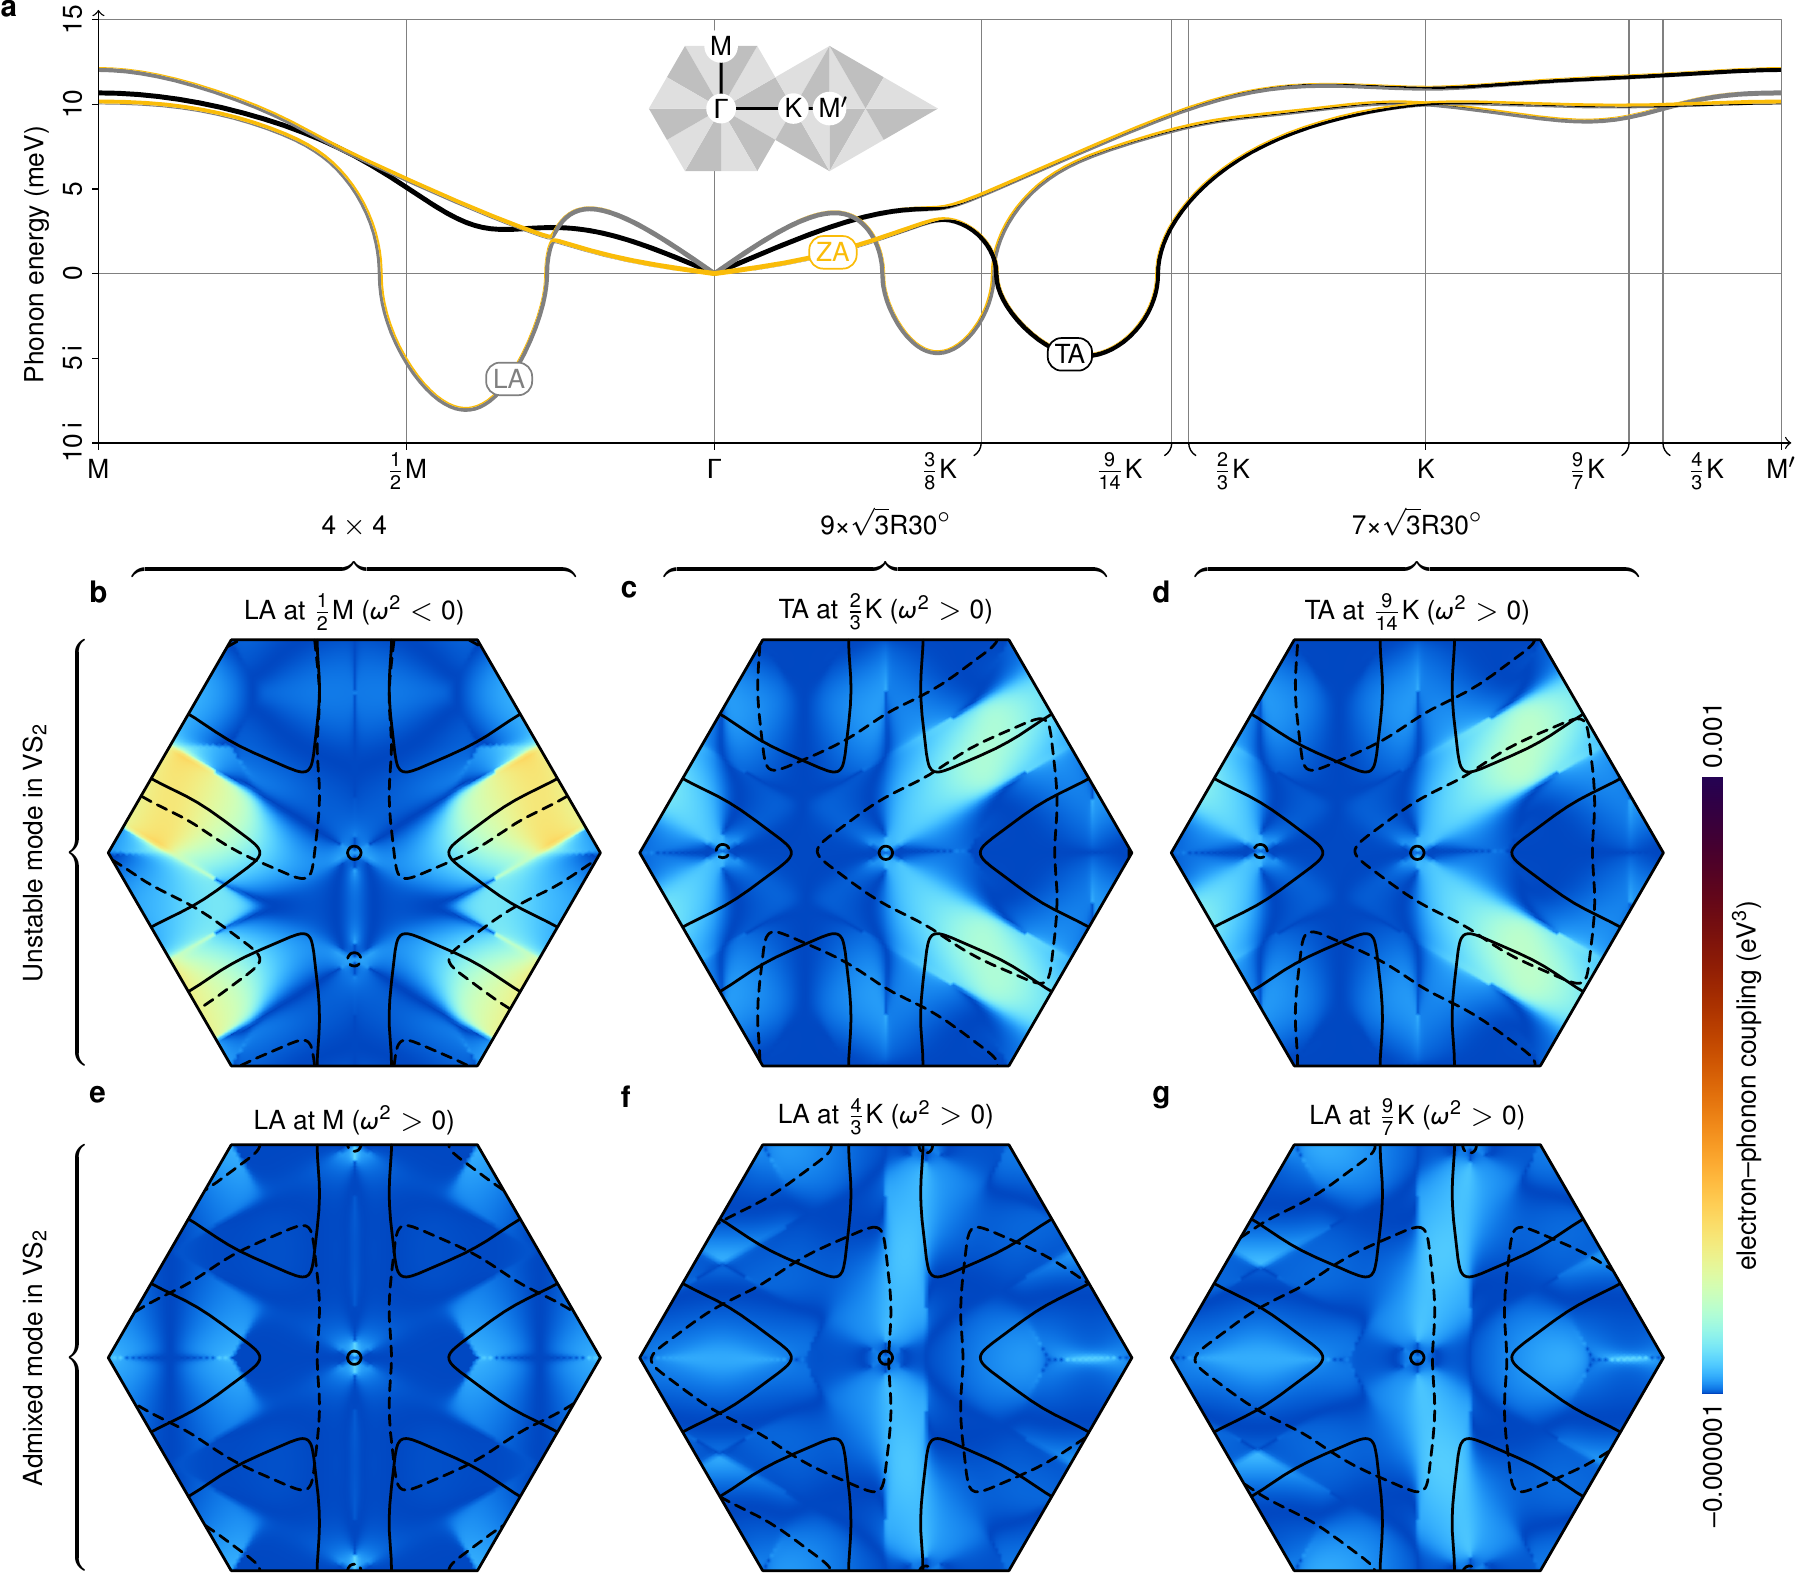}
\caption{\textbf a~Phonon dispersion of monolayer 1T-\vte. \textbf{b--g}~Corresponding electron--phonon coupling $2 \omega_{\vec q} g_{\vec k + \vec q, \vec k} \widetilde g_{\vec k, \vec k + \vec q}$ together with the $\vec k$ and $\vec k + \vec q$ Fermi surfaces (cf.~Fig.~\ref{fig:FSN}).}
 \label{fig:VTe2}
\end{figure*}

\noindent
The phonon dispersion of monolayer 1T-\vte{} obtained from DFPT is shown in Fig.~\ref{fig:VTe2}a. We find similar lattice instabilities as in the case of 1T-\va{} (cf.~Fig.~2a of the main text), albeit shifted to smaller $|\vec q|$. This shift, which is more pronounced for the transverse--acoustic instability in the $\overline{\Gamma \mathrm K}$ direction than for the longitudinal--acoustic instability in the $\overline{\Gamma \mathrm M}$ direction, can be traced back to differences in the Fermi surface (topology) rather than in the electron--phonon coupling, see Fig.~\ref{fig:VTe2}b--g: Instead of the cigar-shaped electron pockets around the $\mathrm M$~points in 1T-\va{} (cf.~Fig.~\ref{fig:FSN}), we find triangular hole pockets around the $\mathrm K$~points (as well as a small hole pocket at $\Gamma$) in 1T-\vte{}. In the latter case, the approximately parallel segments of the Fermi surface are closer together.

\pagebreak

\section*{Table~\ref*{tab:energy_gains}: CDW energy gains in \va{} vs \vte}

\begin{table*}[h!]
  \begin{center}
    \caption{Comparison of maximum atomic displacements and energy gains upon CDW formation for different materials and periodicities from DFT (PBE). All energies refer to a single V$X$\textsubscript2 unit; the reference for the displacements is the lattice constant.}
    \label{tab:energy_gains}
    \begin{tabular}{l|rr|rr}
      & \multicolumn{2}{c|}{1T-\va} & \multicolumn{2}{c}{1T-\vte} \\
      \hline
      \4 & \SI{4}{\%} & \SI{3.4}{\meV} & \SI{13}{\%} & \SI{34.2}{\meV} \\
      \7 & \SI{8}{\%} & \SI{22.7}{\meV} & \SI{6}{\%} & \SI{2.5}{\meV}
    \end{tabular}
  \end{center}
\end{table*}

\noindent
To compare the energy gains associated with CDW formation in 1T-\va{} and in 1T-\vte{} for the different periodicities, we performed structural relaxations on corresponding supercells in the framework of DFT (PBE). The energy gains reported in Table~\ref{tab:energy_gains} show that in 1T-\va{} the \7 CDW is favored over the \4 CDW; in 1T-\vte{} vice versa. The DFT prediction is thus in line with experimental observation for both materials.

\pagebreak

\section*{Figure~\ref*{fig:compression}: Compression of electronic spectrum}

\begin{figure*}[h!]
\centering
\includegraphics[width=0.7\columnwidth]{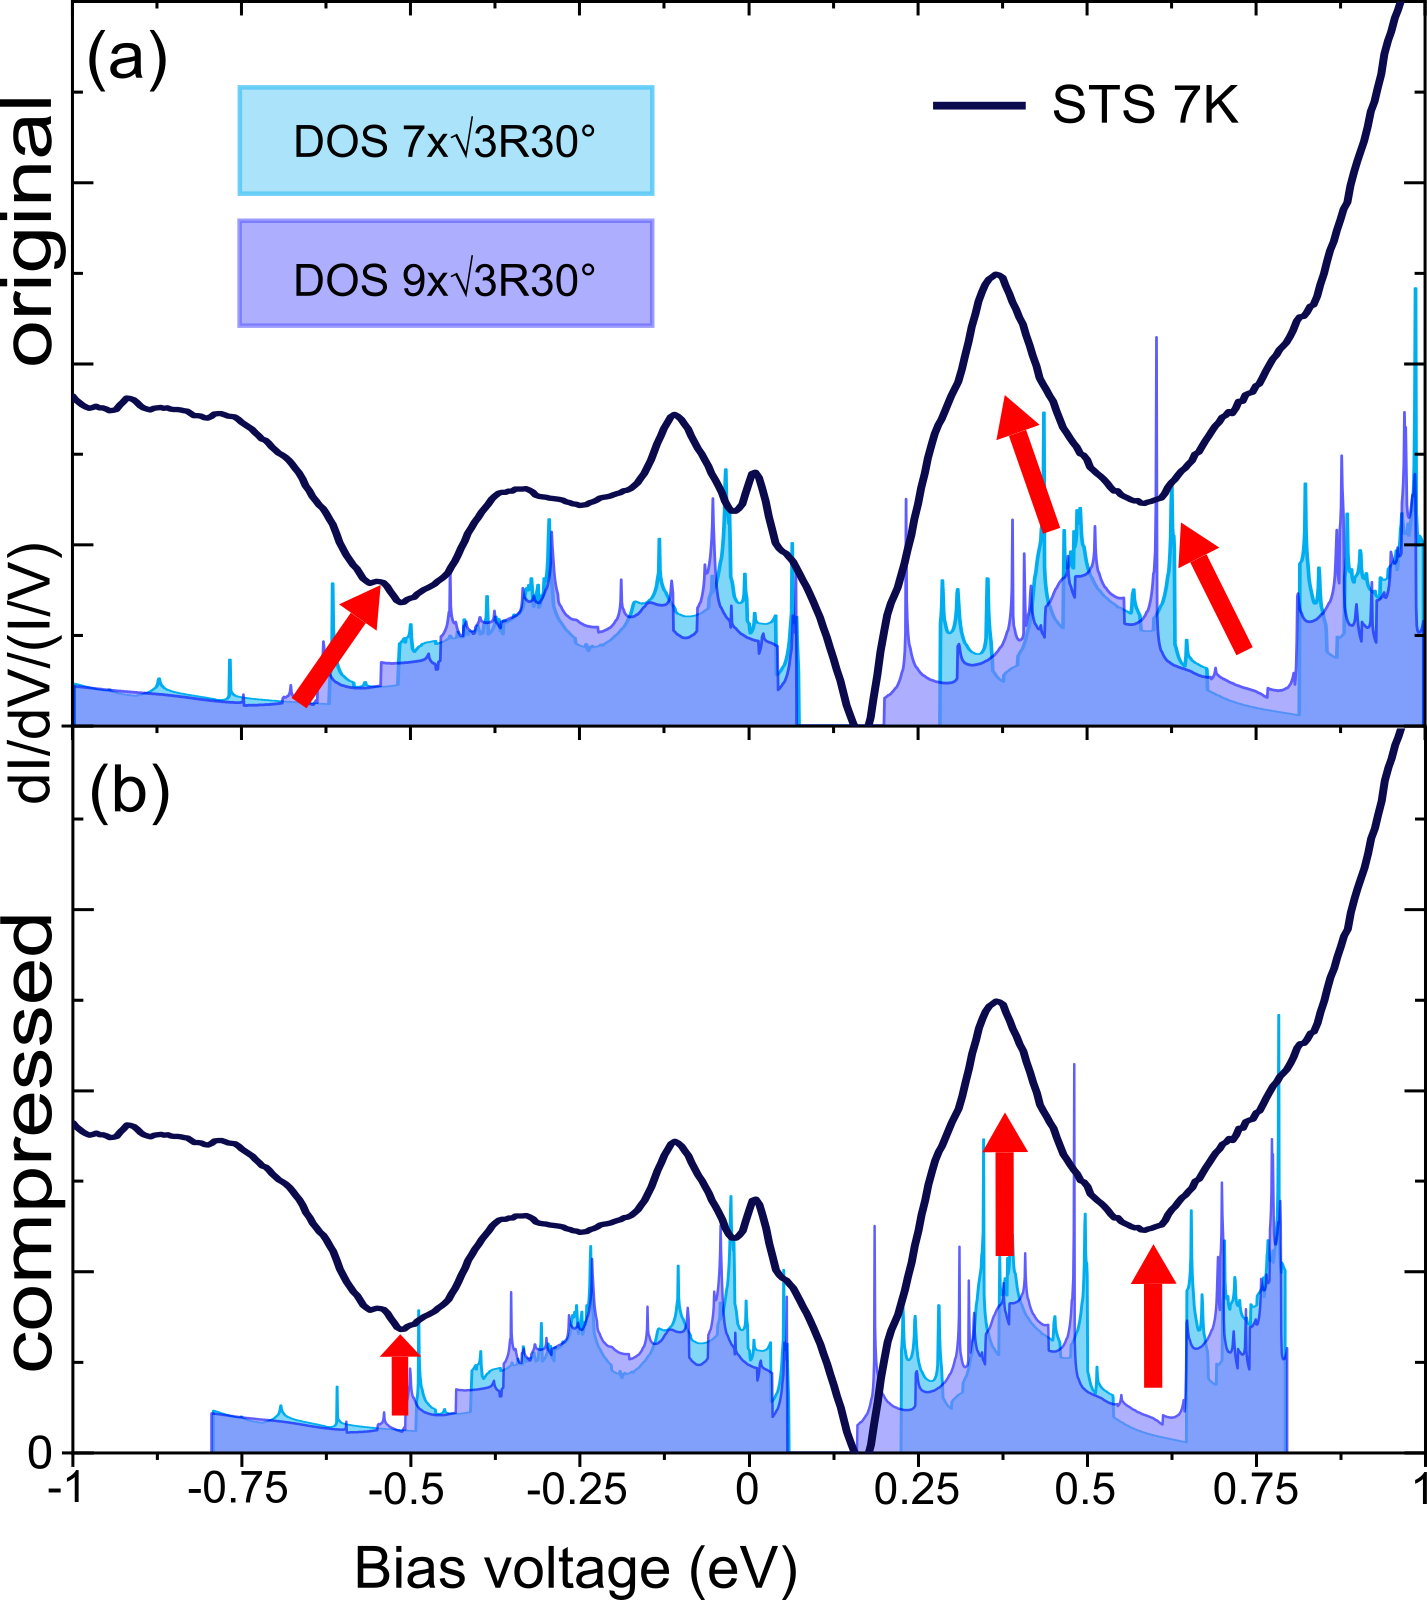}
\caption{Compression of experimental spectrum relative to DFT-calculated DOS\@. In \textbf a, the \SI{7}{\kelvin} spectrum from the main manuscript is compared to the calculated DOS for the \7 and \9 unit cells. In \textbf b, the calculated DOS is compressed to about \SI{80}{\%} of its original width. The red arrows in \textbf{a,\,b} indicate three major features in the spectrum and DOS that can be harmonized between them when the DOS is compressed.}
 \label{fig:compression}
\end{figure*}

\noindent
In Fig.~4a of the main text, the DOS from DFT appears to be wider than the experimental spectrum. Dynamic electronic correlation effects beyond DFT are a possible source of this discrepancy, since they can lead to band renormalization\cite{Giuliani2005}. More precisely, they effect a mass enhancement of the electrons, i.e., the quasi-particle dispersions become flatter than what is expected from theories like DFT\@. In the case of purely local correlations\cite{Georges1996}, this effect is described by a single renormalization factor $Z$ or the corresponding mass enhancement factor $1 / Z$. Figure~\ref{fig:compression} shows that we obtain a good match between experimental and theoretical spectra by setting $Z = 0.8$. This is indicative of moderate electronic correlations. For comparison, examples range from diverging mass enhancement at Mott--Hubbard transitions, via mass enhancement factors of about 10 to 1000 in Kondo or heavy fermion systems, to enhancement factors between 1 and 10 in transition-metal compounds like metallic chromium or iron-based superconductors. The mass enhancement factor of $1 / Z \approx 1.25$ puts \va{} at similar electronic correlation strengths as, e.g., metallic chromium\cite{Qazilbash2009}.

The rise in the normalized \dIdV{} beyond \SI{-0.5}{\eV} can be attributed to contributions from the graphene/Ir(111) substrate, which can come to dominate the signal for large $V$ when the \va{} has a small DOS\@. In this case, the graphene spectrum (not shown) diverges beyond the Ir(111) surface state at \SI{-190}{\meV}.

\pagebreak

\section*{Figure~\ref*{fig:dIdV maps FFT}: Suppression of CDW Fourier intensity within the gap}

\begin{figure*}[h!]
\centering
\includegraphics[width=\columnwidth]{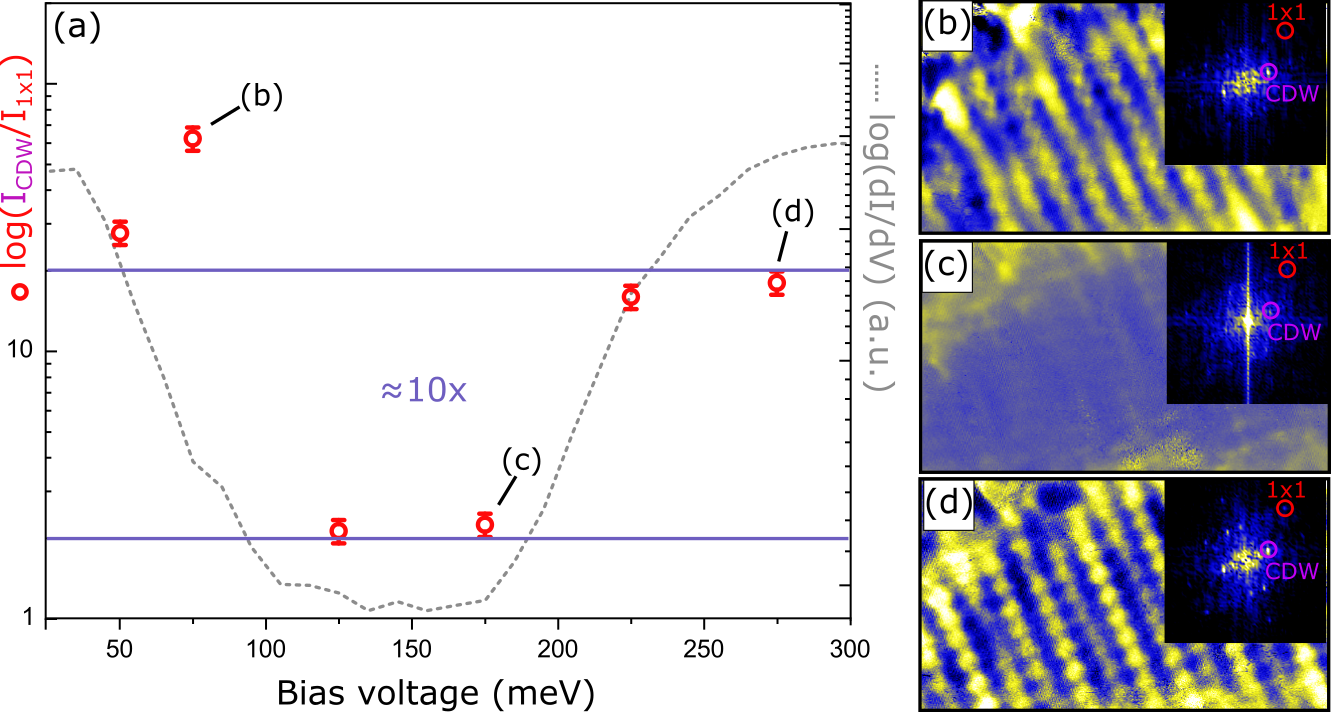}
\caption{Suppression of CDW within the gap. \textbf a~Logarithmic plot of the CDW intensity in the Fourier transform of \dIdV{} conductance maps, normalized to the $1 \times 1$ lattice intensity. Additionally, a \dIdV{} spectrum is plotted in order to indicate the location and width of the gap. \textbf{b--d}~\dIdV{} conductance maps taken at the voltages indicated in \textbf a. Measurement settings: (maps) \SI[parse-numbers=false]{9.5 \times 5.5}{\nano\meter\squared}, $I_{\text{t}} = \SI{0.3}{\nano\ampere}$, except for the map at \SI{50}{\meV}, which is taken at $I_{\text{t}} = \SI{0.6}{\nano\ampere}$; (\dIdV{} spectrum) $f = \SI{777.7}{\Hz}$, $I_{\text{t}} = \SI{0.4}{\nano\ampere}$, $V_{\text{r.m.s.}} = \SI{6}{\meV}$. All data taken at $T = \SI{7}{\kelvin}$.
}
 \label{fig:dIdV maps FFT}
\end{figure*}

\noindent
Apart from the different charge distributions on either side of the gap discussed in the main manuscript, \dIdV{} maps taken within the gap show a clear suppression of the CDW\@. For a quantitative analysis, we have Fourier analyzed the \dIdV{} maps and normalized the CDW peak in the Fourier spectrum with respect to the \1 lattice peak intensity. The resulting value $R = I_{\text{CDW}}/I_{1 \times 1}$ is observed to fall by an order of magnitude within the gap. Since a gap of other than CDW origin would have the same value of $R$ in- and outside of the gap region\cite{Ugeda2016}, this is another clear indication of the relation between gap and CDW\@.

\pagebreak

\section*{Figure~\ref*{fig:bands_extended}: Bands along extended Brillouin-zone path}

\begin{figure*}[h!]
\centering
\includegraphics[width=\linewidth]{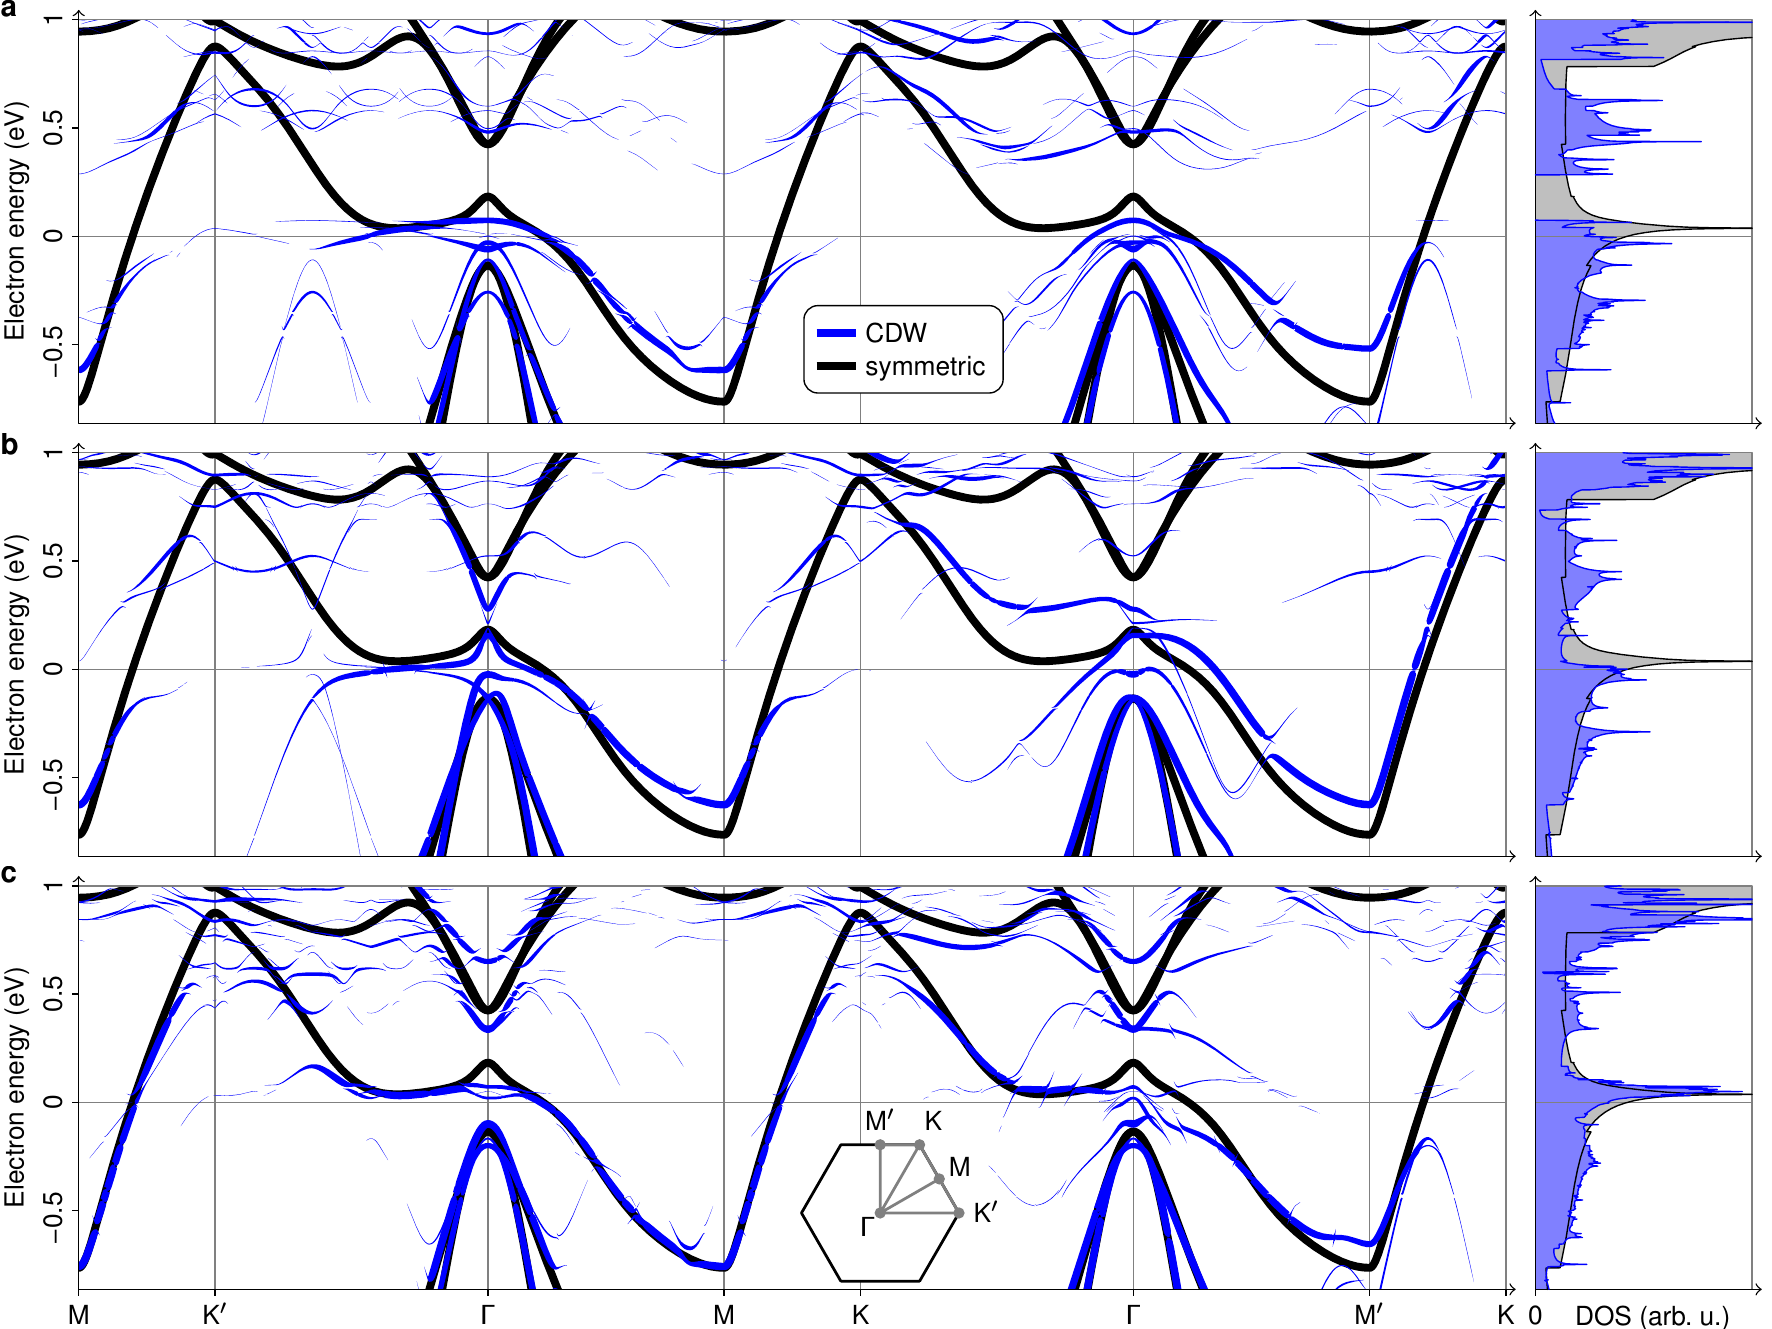}
\caption{Electronic band structure along an extended Brillouin-zone path and DOS of monolayer 1T-\va{} for \textbf a~the full \7 CDW displacements, \textbf b their projection onto unstable phonon modes, and \textbf c the orthogonal complement.}
 \label{fig:bands_extended}
\end{figure*}

\noindent
In Fig.~5a of the manuscript, we show the electronic band structure of monolayer 1T-\va{} in the \7 phase along a selected high-symmetry path $\Gamma$--$\mathrm M$--$\mathrm K$--$\Gamma$ of the undistorted phase only. Once the distortion breaks the C\textsubscript3 symmetry, this path is not representative of the full Brillouin zone anymore. For completeness, in Fig.~\ref{fig:bands_extended}a, we thus reproduce the respective data along an extended path, again supplemented with the DOS\@. In Fig.~\ref{fig:bands_extended}b,\,c, we show the analogous results for the projection of the displacement onto the soft transverse--acoustic phonon modes at $\vec q = \pm 9/14\,\overline{\Gamma \mathrm K}$ and the orthogonal complement. There are some salient differences between the electrons for the full and partial CDW displacement. In Fig.~\ref{fig:bands_extended}b, the gap between $\mathrm M'$ and $\mathrm K$ is missing; in turn, in Fig.~\ref{fig:bands_extended}c, there is no gap between $\mathrm M$ and $\mathrm K'$ as well as $\mathrm M$ and $\mathrm K$. The combination of both displacement components is needed to open a full gap.

\pagebreak

\section*{Figure~\ref*{fig:avoided_crossing}: Preservation of states at the Fermi level}

\begin{figure*}[h!]
\centering
\includegraphics[width=\linewidth]{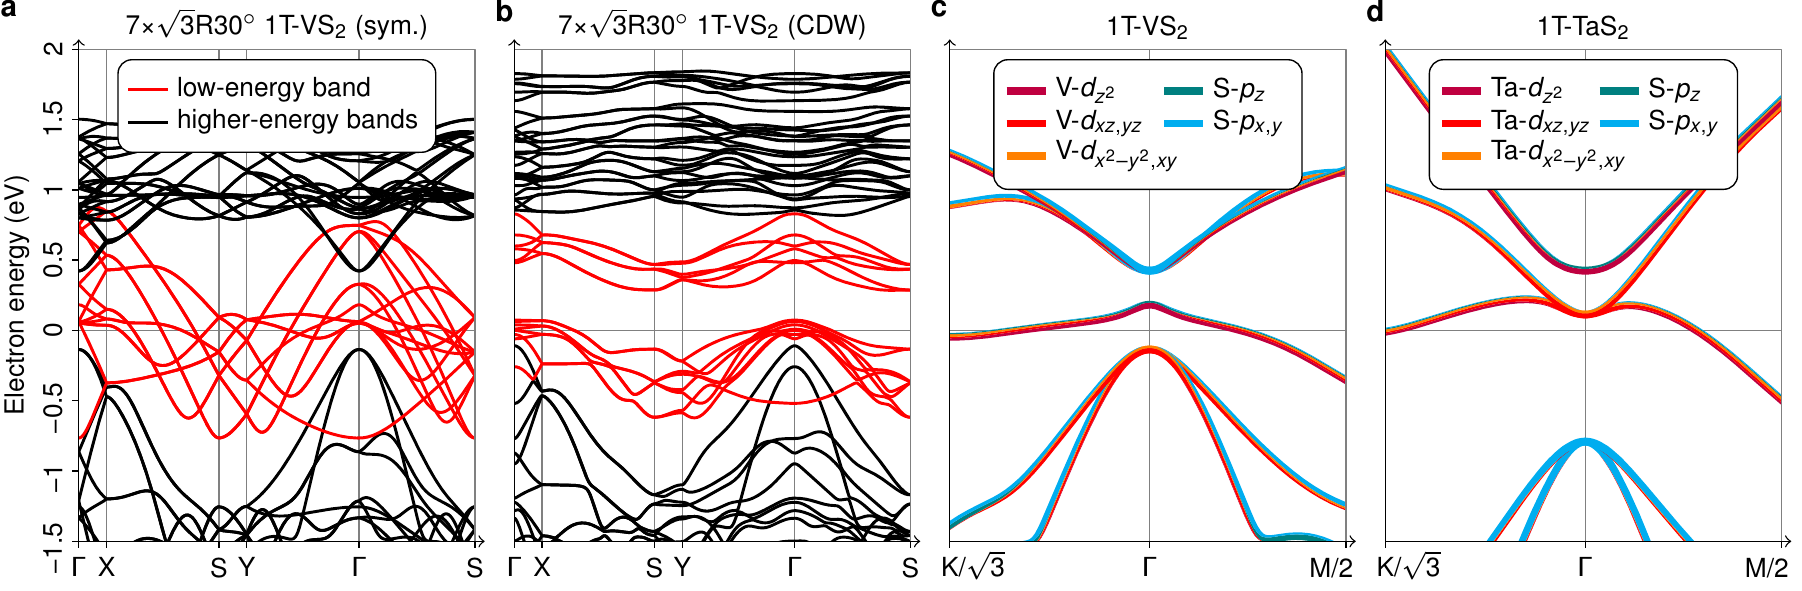}
\caption{\textbf{a,\,b}~Band structure of symmetric and distorted 1T-\va{} along path through Brillouin zone corresponding to \7 cell. The low-energy band is half-filled and splits into seven four-fold (including spin) bands between $\mathrm X$ and $\mathrm S$. Thus, there must be 1/7 unoccupied states per V~atom below the gap. \textbf{c,\,d}~Orbital-resolved low-energy electron dispersion of 1T-\ta{} and 1T-\va{} near $\Gamma$. In the case of 1T-\va{} there is an avoided crossing between V-$d$ and S-$p_{x, y}$ bands.}
\label{fig:avoided_crossing}
\end{figure*}

\noindent
The CDW does not create a complete gap at the Fermi level. For the commensurate structures used to approximate the incommensurate CDW, it is the combination of the electron count and the symmetry of the unit cell that guarantees a partially filled band, i.e., a metallic DOS\@. A complete gap at the Fermi level in the CDW would require the splitting of bands that must be degenerate by symmetry of the CDW structures (Fig.~\ref{fig:avoided_crossing}a,\,b), i.e., further symmetry breaking.

The particular form of the remaining spectral weight at the Fermi level resembling a downwards dispersing parabola around $\Gamma$ in the CDW state (cf.~Fig.~5) can be understood in terms of orbital band characters: In 1T-\va{}, we find an avoided crossing of V-$d$ and S-$p_{x, y}$ bands in the relevant region and thus a signification hybridization between these states (Fig.~\ref{fig:avoided_crossing}c). This is opposed to, e.g., the case of 1T-\ta, where the S-$p_{x, y}$ states are much lower in energy (Fig.~\ref{fig:avoided_crossing}d). Now, while the $d$-type bands are heavily reconstructed due to the CDW, the $p$ orbitals are less affected and can contribute to a new Fermi surface in the case of 1T-\va{} in contrast to 1T-\ta.

\pagebreak

\section*{Figure~\ref*{fig:VS2 XMCD}: XMCD sample morphology}

\begin{figure*}[h!]
\centering
\includegraphics[width=0.5\columnwidth]{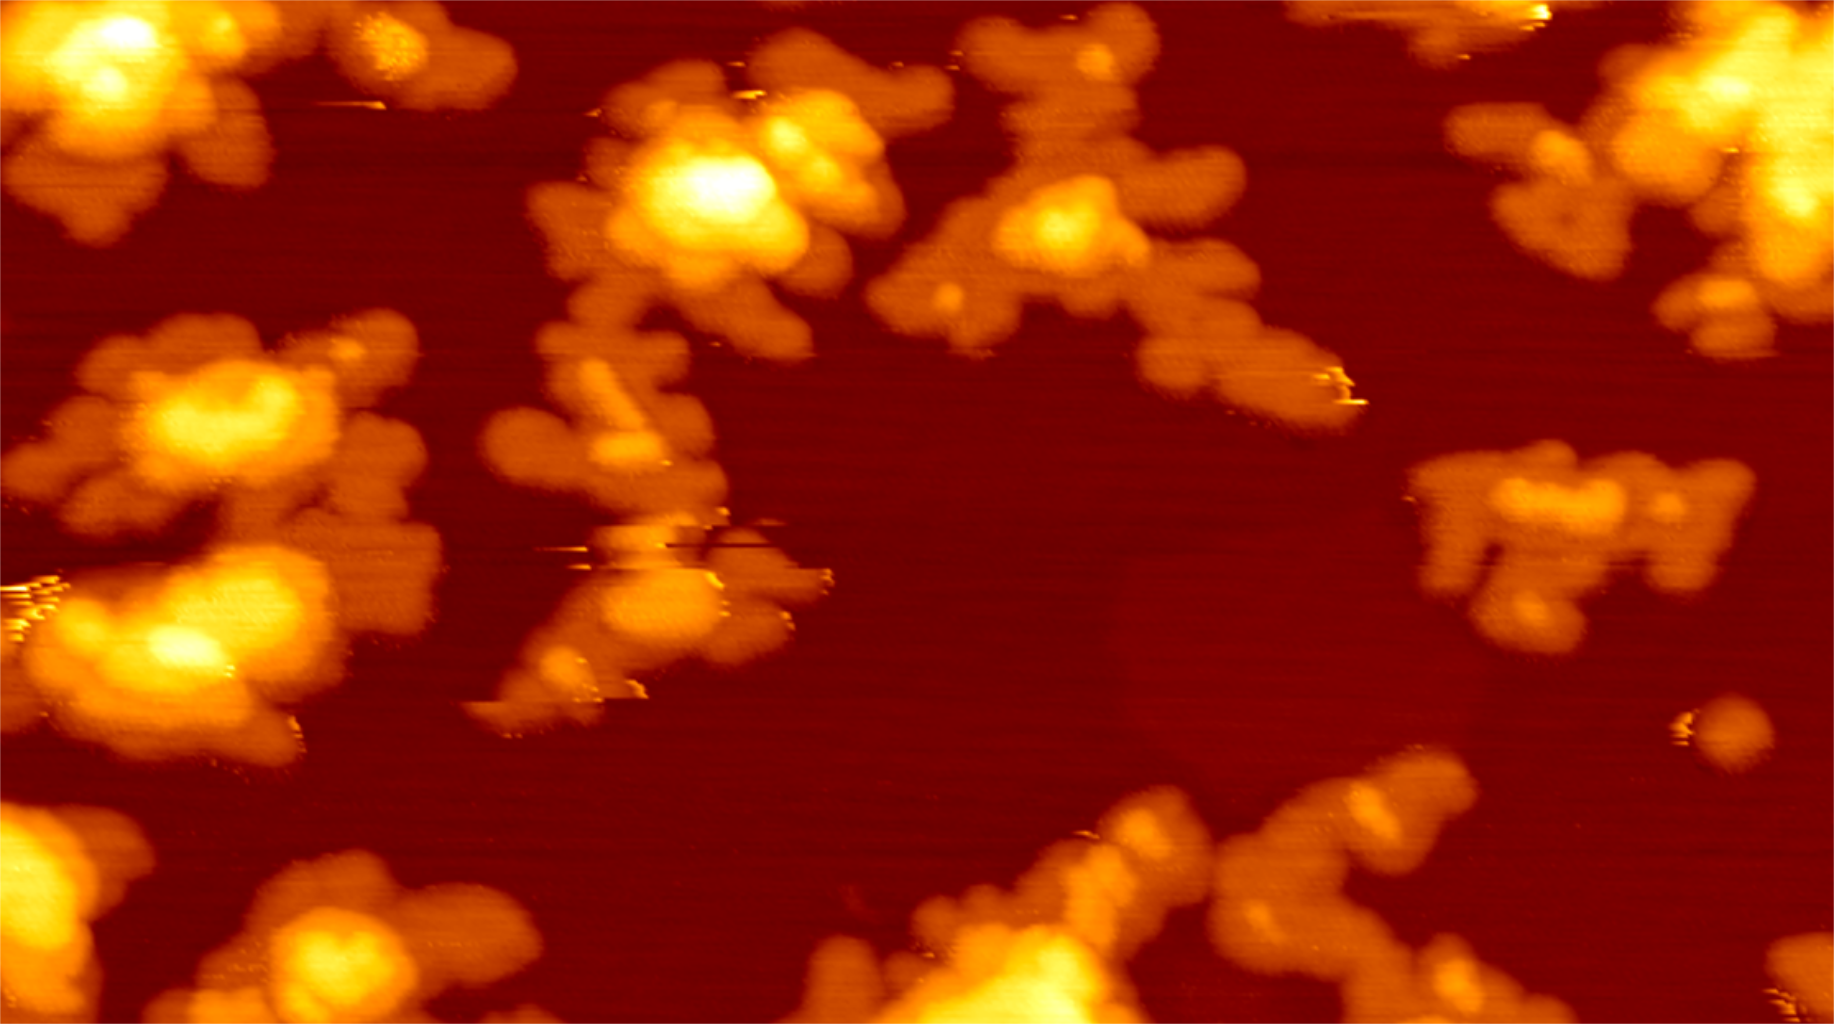}
\caption{Magnetic properties of \va: STM topograph illustrating the sample morphology of the XMCD measured sample. Image size:~\SI[parse-numbers=false]{100 \times 50}{\nano\meter\squared}.}
 \label{fig:VS2 XMCD}
\end{figure*}

\noindent
In the main manuscript, we describe the magnetic properties of \va{} as measured by x-ray absorption spectroscopy (XAS) and x-ray magnetic circular dichroism (XMCD). Figure~\ref{fig:VS2 XMCD} displays the sample morphology of the investigated sample. Like the samples shown in the main text, the island shape is dendritic. By comparison to substrate step edges, the monolayer height is measured to be \SI{7}{\angstrom}. The sample has a monolayer coverage of about \SI{40}{\%}. Distinct height levels indicate three layers.

\pagebreak

\section*{Figure~\ref*{fig:SDW}: DOS for SDW}

\begin{figure*}[h!]
\centering
\includegraphics[width=0.7\linewidth]{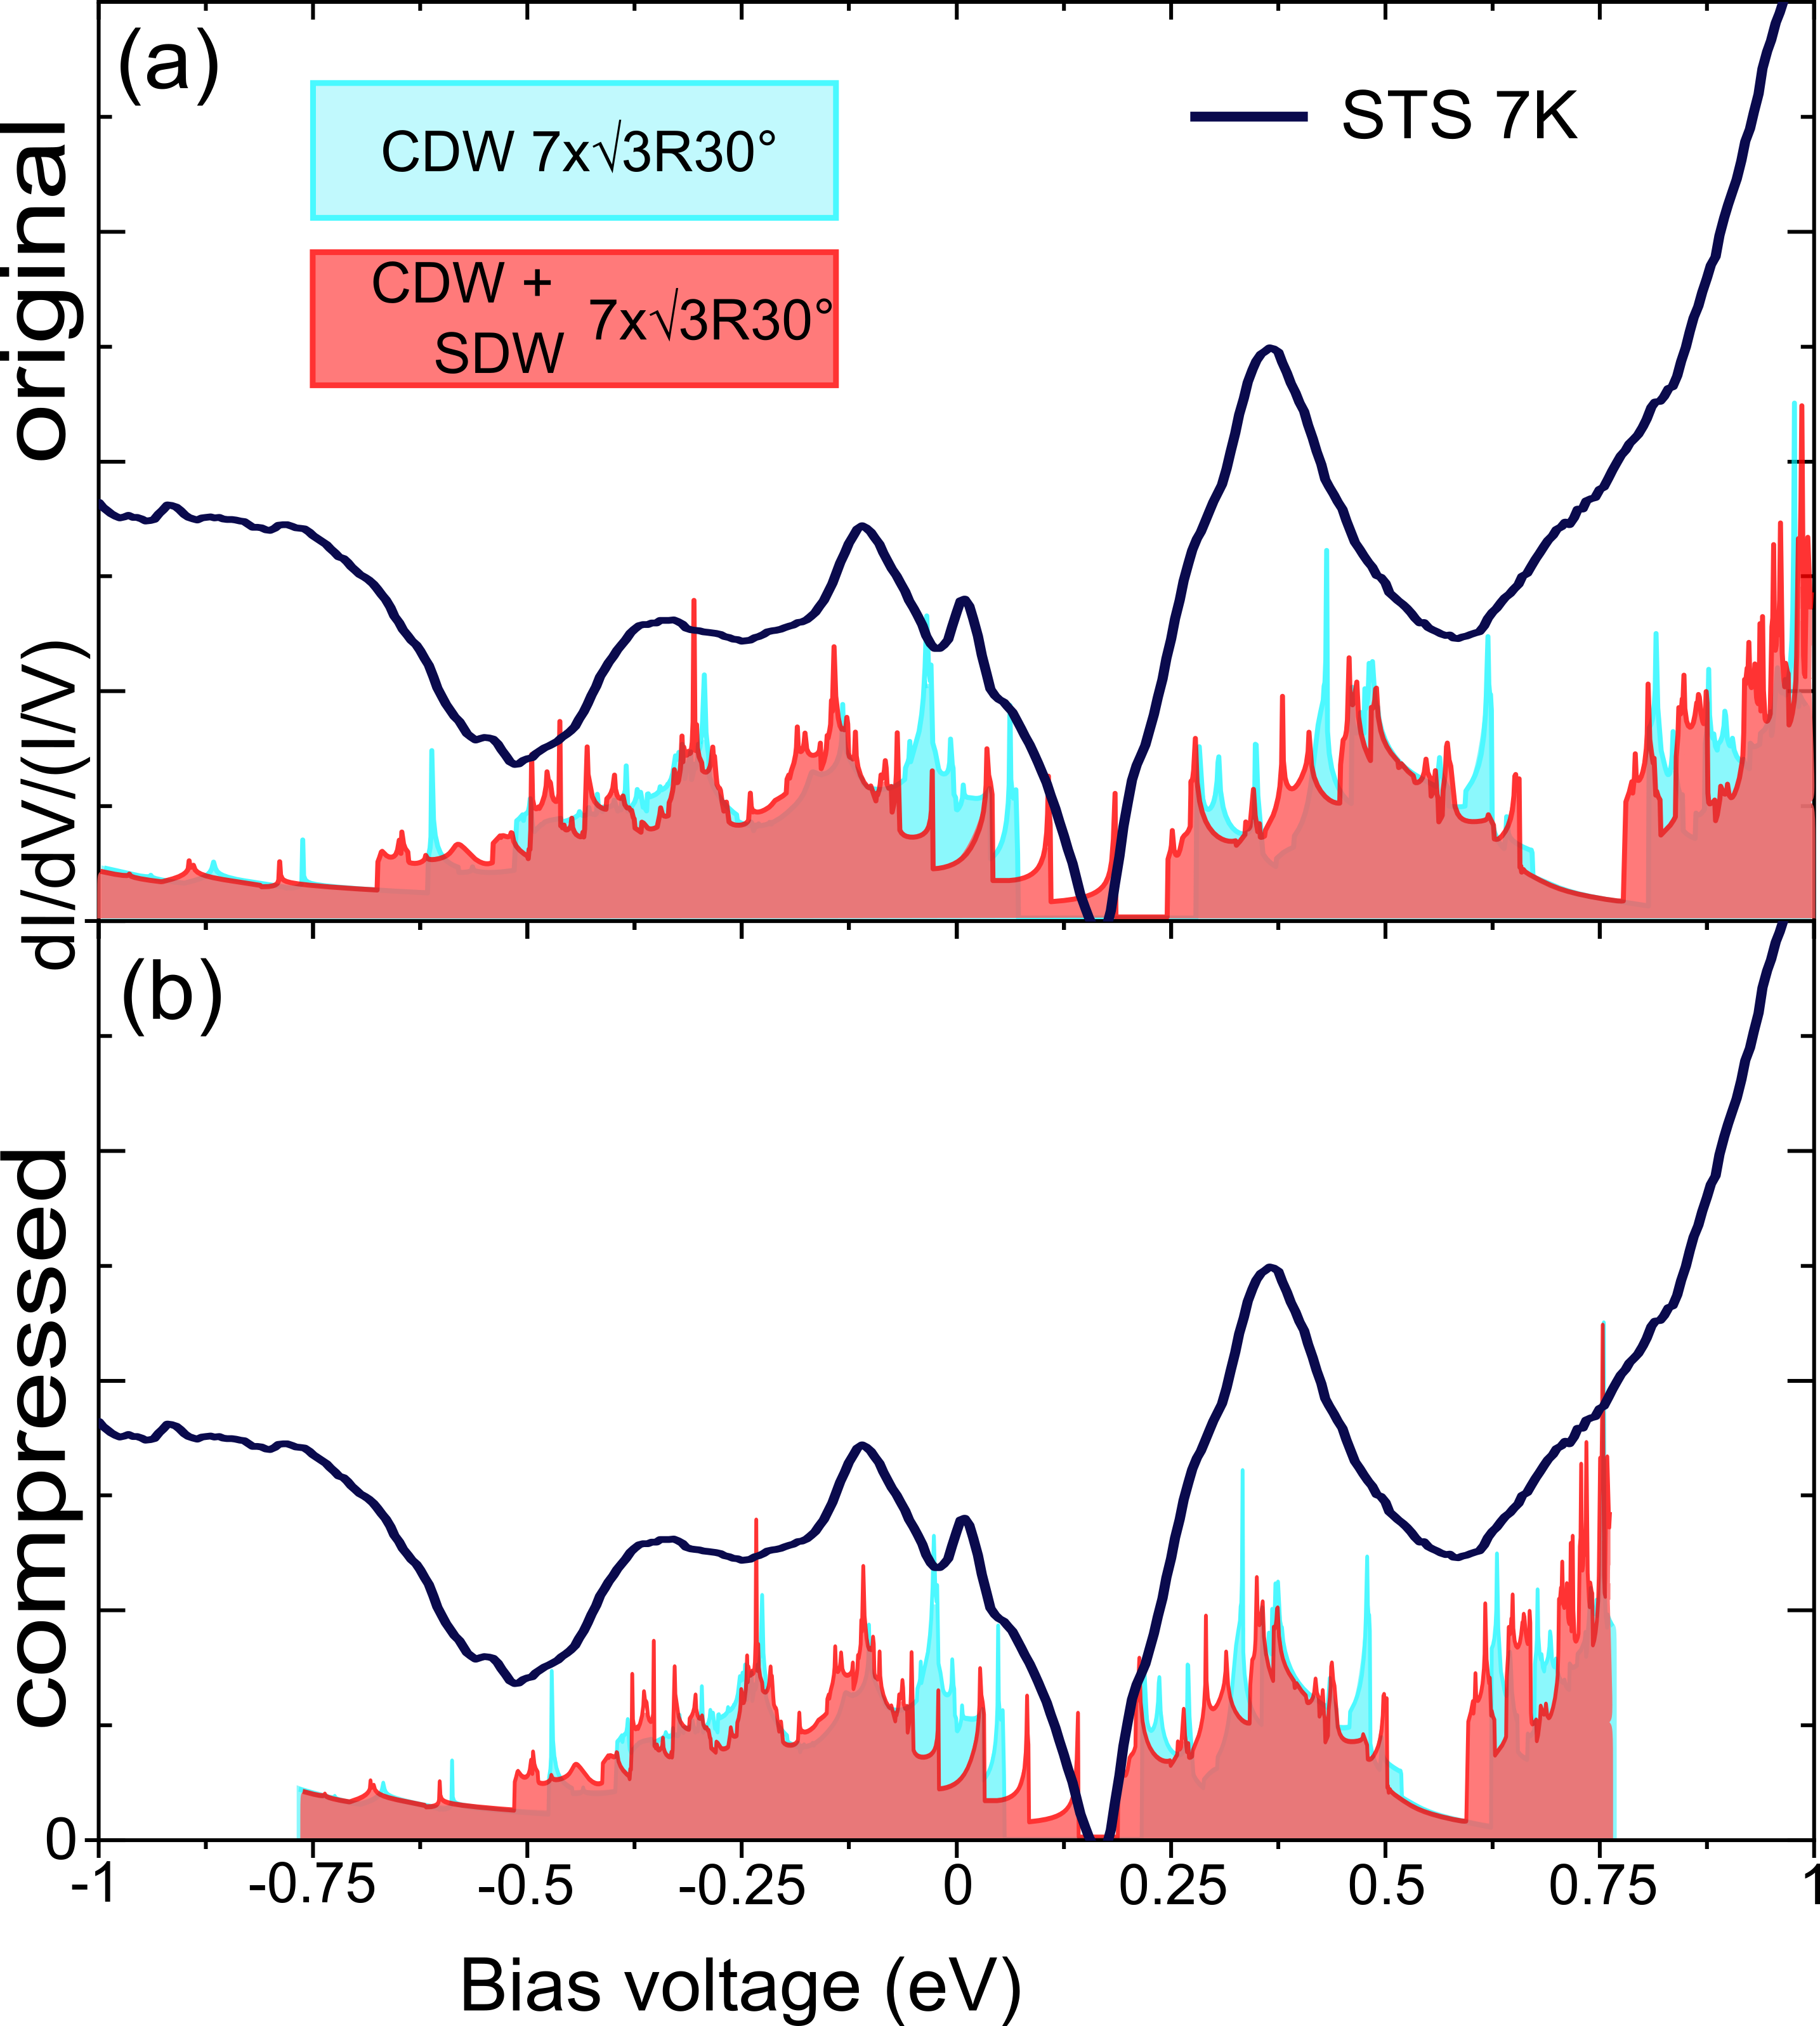}
\caption{\textbf{a}~\dIdV{} spectra taken with a Au tip on monolayer \va{} at \SI{7}{\kelvin} along with DFT calculated CDW DOS with (red) and without (cyan) SDW\@. \textbf{b}~The same data after compressing calculated DOS to 80\% of original size.}
\label{fig:SDW}
\end{figure*}

\noindent
In Fig.~\ref{fig:SDW}a, we show the DOS of the CDW structure with and without spin density wave (SDW), along with the experimental \dIdV{} spectra. The most prominent difference in the DOS is the reduction of the gap size. For the \7 structure, the gap shrinks from  \SI{0.21}{\eV} to \SI{0.06}{\eV} when the CDW is coupled to a SDW\@. Since the CDW gap is indeed much larger in DFT than the experimental gap, this can be considered as an additional argument for the simultaneous presence of a SDW\@. Taking into account the compression of the experimental data, discussed under Fig.~\ref{fig:compression}, the DOS of the coupled CDW--SDW is in even better agreement with the experimental spectra, as seen in Fig.~\ref{fig:SDW}b.

\pagebreak

\section*{Figure~\ref*{fig:FS_VSe2}: Comparison of DFT results with literature data for VSe2}

\begin{figure*}[h!]
\centering
\includegraphics[width=\linewidth]{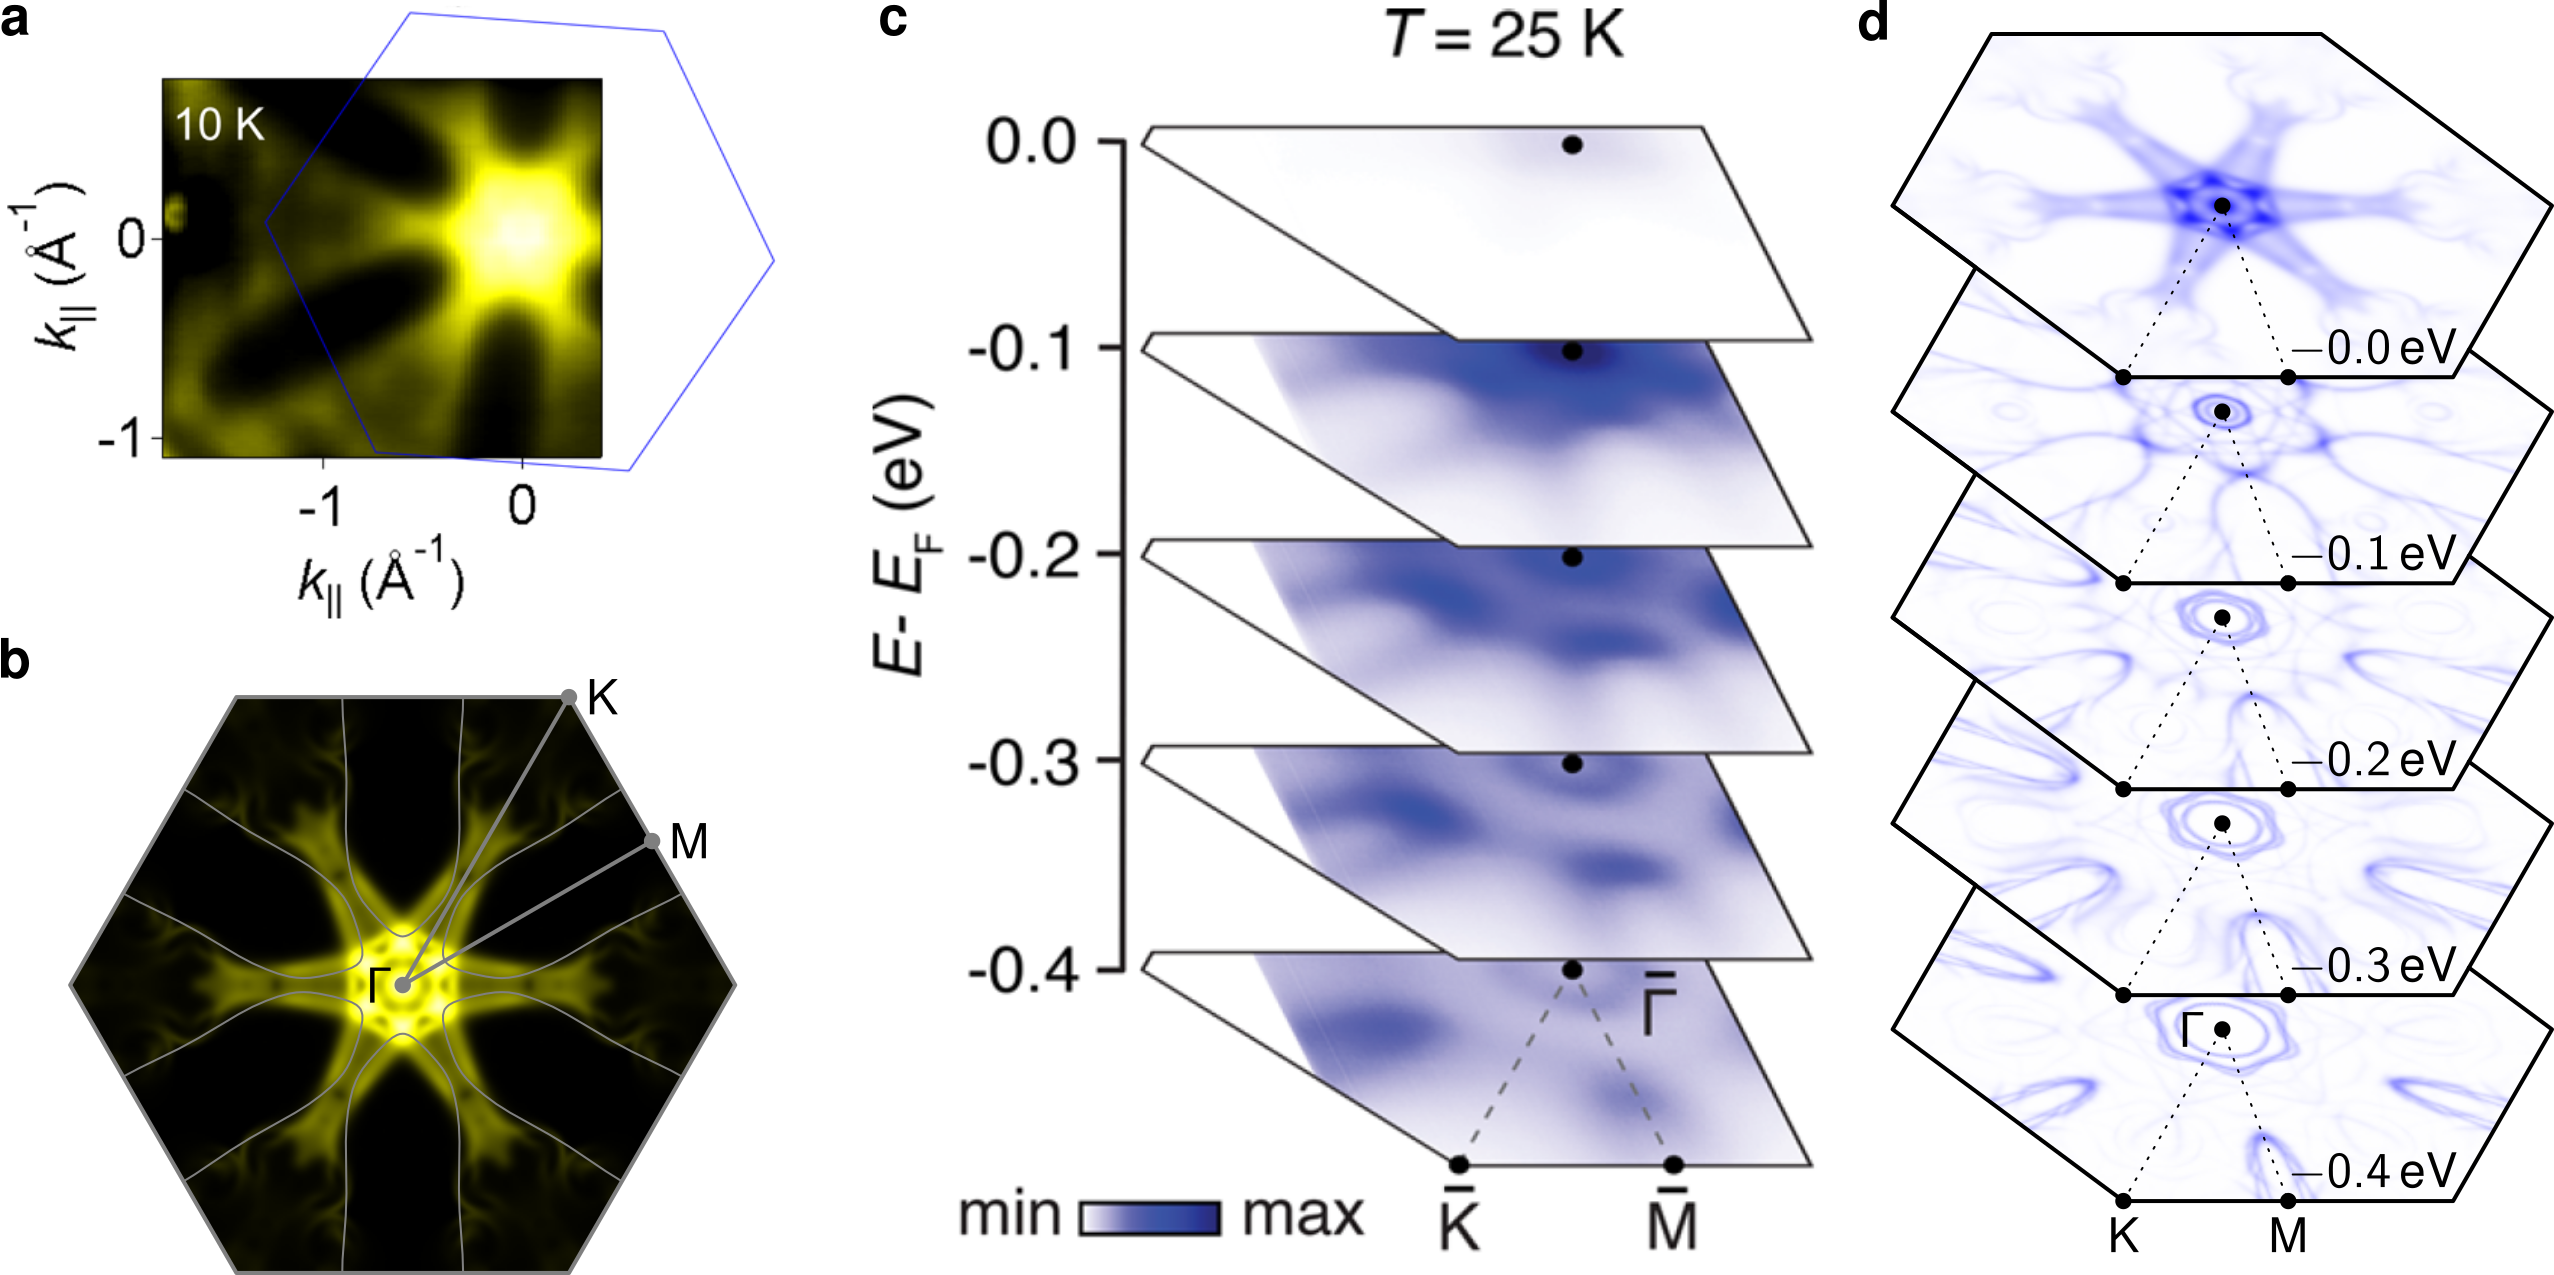}
\caption{Fermi surface of \7 CDW of monolayer 1T-\ve{} averaged over regions of different CDW orientations and comparison to experiment. \textbf a~Fermi surface reprinted with permission from Ref.~\citenum{Chen2018} \copyright~2018 American Physical Society. \textbf b~Symmetrized Fermi surface calculated in this work. \textbf c~Energy isolines reprinted with permission from Ref.~\citenum{Feng2018} \copyright~2018 American Chemical Society. \textbf d~Symmetrized energy isolines calculated in this work.}
\label{fig:FS_VSe2}
\end{figure*}

\noindent
In order to compare our DFT results for monolayer \ve{} to existing ARPES studies, we have averaged our calculated Fermi surface of \ve{} in the \7 CDW phase over all domains of the CDW with respect to the lattice. In this way, many of the familiar ARPES characteristics of \ve{} are uncovered. If we compare to \ve{} systems where only the \7 CDW was observed\cite{Chen2018, Coelho2019}, we see that the experimental data in Fig.~\ref{fig:FS_VSe2}a, taken from Ref.~\citenum{Chen2018}, shows excellent agreement with our calculated Fermi surface in Fig.~\ref{fig:FS_VSe2}b. In particular, we observe the formation of gaps between $\mathrm M$ and $\mathrm K$, while the rest of the Fermi surface remains intact. The apparent persistence of the six cigar-shaped electron pockets and the appearance of the hole pocket around $\Gamma$ are visible in both theory and experiment. That the ARPES measurements show such small changes during the transition to the CDW phase can therefore be understood as stemming mostly from the fact that it is an averaging technique. More subtle changes to the band structure around $\Gamma$ and the elliptic electron pockets cannot easily be compared by eye. All in all, our theoretical studies match very well to experimental ARPES reports of \ve{} in the \7 phase\cite{Chen2018, Coelho2019}.

It must however be noted that most publications on \ve{} find, in contrast to our prediction, a full gap at the Fermi level\cite{Wong2019, Feng2018, Duvjir2018, Chua2020}. Monolayer \ve{}, especially in the light of recent works\cite{Chua2021, Zong2021, Duvjir2021}, seems to have a strong substrate-dependence. It is therefore likely that our calculation, which is based on freestanding \ve{}, does not capture the intricacies of all experimental systems. At the Fermi surface, an (additional) $4 \times 1$ CDW found on some substrates\cite{Duvjir2018, Chua2020, Chua2021, Duvjir2021}, might induce an insulating state. A possible cause for the presence of different and competing CDW orders might be substrate-induced strain\cite{Si2020}, which is not included in our DFT calculations. Fig.~\ref{fig:FS_VSe2}c shows the Fermi surface and constant-energy contours at higher binding energies of a \ve{} system where the Fermi surface is fully gapped at \SI{25}{\K}, taken from Ref.~\citenum{Feng2018}. In this case, though our calculation in Fig.~\ref{fig:FS_VSe2}d does not predict the fully gapped surface, we see that it captures the features of the band structure away from the Fermi level quite well. The dissimilarities between \ve{} systems with different CDW orders might therefore pertain mostly to the Fermi surface and the unoccupied states.

\pagebreak

\bibliographystyle{naturemag}
\bibliography{supplement}
\end{document}
